# Supplementary material for: Deep Data Density Estimation through Donsker-Varadhan Representation
Source: arXiv:2104.06612 source file (2021-04-14)
Supplement: Supplementary file 1 [file 8appendix.tex]

\section{Relationship to GAN}
Generative Adversarial Network (GAN) \cite{goodfellow2014generative} is an unsupervised learning method to generate the data from the prior distribution. 
A GAN model consists of two neural network based models, generator $G$ and discriminator $D$.
The generator tries to generate the data that lies in the distribution of the training dataset.
Whereas the discriminator tries to discern whether the given datapoint is from the training dataset or generated by the generator.
Formally, the loss function of GAN is the following minimax game,

\begin{equation}\label{eq:gan}
    \min_G \max_D V(D,G) = \mathbb{E}_{\mathbf{x}\sim p(\mathbf{x})}[\log D(\mathbf{x})] + \mathbb{E}_{\mathbf{z}\sim p_z(\mathbf{z})}[\log(1-D(G(\mathbf{z})))]
\end{equation}
where $\mathbf{x}$ and $\mathbf{z}$ are instances from the empirical data distribution $p(\mathbf{x})$ and the prior distribution $p_\mathbf{z}(\mathbf{z})$ over predefined space, respectively.
The dimension of the prior distribution space is basically smaller than that of the data. 
Normally, the uniform distribution or the normal distribution are used as the prior distribution.
In the equation above, the discriminator aims to generate the scalar output representing the probability of being a datapoint from the training dataset.
Thus, the output $1$ of $D$ represents that the given datapoint is from the true distribution of the training dataset whereas the output $0$ represents the generated datapoint from $G$.
With respect to the parameters in $D$, the loss function of GAN can be regarded as minimizing the binary cross entropy.
Also, the generator $G$ aims to disturb $D$ to not discern the datapoint well.
After training, it is expected that the generator generates the datapoints following the true probability distribution.

GAN aims to generate the data given the prior distribution, mainly focused on the generator, which is sometimes called deep generative model because it tries to generate the data.
However, we directly estimate the data density by the neural network based model, whereas GAN generates the generator that can map from the prior to the desired data space. 

Also, please make sure that GAN uses two different models; the generator and discriminator, however, DDDE needs one model for both generated samples from the uniform distribution and the samples from the data, which leads to more stable training because it does not involve any minimax formulations as GAN uses that usually suffers from instability and oscillation during the training.

\section{Proofs on the theoretical properties}
